# Supplementary material for: Planning profitable tours for field sales forces: A unified view on sales analytics and mathematical optimization
Source: arXiv:2011.14822 source file (2020-11-27)
Supplement: Supplementary file 1 [file 09_appendix.tex]

\pagebreak

\section{Appendix}

\section*{Related Work}

\subsection*{Problem description}

Given are a planning horizon including several weeks (4 in our case) and a set of customers, comprising both optional and mandatory customers.
Mandatory customers have to be visited during the planning horizon.
Each customer is assigned a visit rhythm and a reward value obtained by each visit at this customer.
If a customer is included in a plan, the visit rhythm has to be respected, i.e., it is not possible to schedule one visit in four weeks for a customer with a visit rhythm of two weeks.
The customers are served by a sales representative within a daily working time window. 
Customers may specify time windows that also have to be respected.

The problem is to select the visited customers, assign customer visits to days and to provide daily tours for the sales representative such that the working time window is respected, all mandatory customers are included in the plan, the visit rhythm is respected, and the total reward is maximal.

\subsection*{Optimization approaches}

In general, we can identify three related models
\begin{itemize}
\item Territory design with a focus on balance and compactness, 
\item Vehicle routing with periodic constraints and (potentially) workload restrictions and balance restrictions, 
\item Orienteering with primary concern of selecting visits given capacity and workload restrictions: 
\end{itemize}

\subsubsection*{Territory design}

Territory design, and specifically service territory design, addresses the problem of planning compact and balanced territories for salespeople, transport service providers, heath service providers etc.
We refer to \cite{Kalcsics2015} for a detailed overview.

While several approaches exist in this line of work, only few publications explicitly address the problem of scheduling customer visits over a planning horizon of several weeks or months.

\cite{Lei2015} introduce the multiple traveling salesman and districting problem with multi-periods and multi-depots (MTSDPMPMD ;-) ?).
The planning horizon is separated into periods, with each period lasting several weeks.
The customers are exactly served once per period. 
In each period, customers are grouped into districts, each of which is assigned to one salesperson. 
In each district, customers are again grouped into one subdistrict per day.
The customers in one subdistrict have to be visited by a single salesperson route subject to route length restrictions.
The objective is to minimize a  weighted linear combination of the number of districts, a compactness measure on the level of subdistricts, a dissimilarity measure for subsequent periods, and a balance measure for the salespersons' profits. 
The authors use an adaptive large neighborhood search (ALNS) for solving instances with up to 400 customers.

To our knowledge, this is the only model that combines a districting and traveling salesman problem in the context of multi-period territory design.
However, it does not consider regularities on the level of customers.
Similar to our setting, information on customer-specific profits is available and a daily duration limit on the salespersons' routes applies.
However, rather than selecting a profit-maximizing subset of customers to visit in case the duration limit is exceeded, the MTSDPMPMD instead penalizes overtime with a linear factor. 

In the multi-period service territory design problem (MPSTDP) introduced in \cite{Bender2016}, customers are grouped into weekly and daily clusters served by one salesperson.
This problem explicitly addresses customers which have to be served several times during the planning horizon subject to day and weekday regularities. 
The aim of this problem is to plan compact clusters subject to balance constraints based on an activity measure, e.g. a workload measure.
In contrast to our model, customers are balanced with respect to the average workload, while a maximum daily workload limit does not apply.
Routing aspects are not explicitly considered in this model. 
The authors propose a location-allocation heuristic for problem instances derived from real-world applications with an average of 115 customers and a planning horizon of 16 weeks.
Additionally, \cite{Bender2018} propose a branch-and-price algorithm for a closely related problem that is able to solve instances with 55 customers and a planning horizon of 4 weeks in reasonable computation times.

\subsubsection*{Vehicle routing problems}

Periodic vehicle routing problem (PVRP) variants address the problem of assigning each customer a visit schedule following a given visit frequency and requested visit regularities.
The problem has been discussed in the context of various practical applications from home health care to service technician routing and waste collection. 
Surveys on these variants and related problems can be found in \cite{Francis2008} and \cite{Campbell2014}. 
Due to the variety of problems in this line of research, we limit this review to the studies closely related to our problem setting. 

A survey on the consideration of (workload) equity in VRPs with and without periodic aspects has been published recently by \cite{Matl2017}.

\cite{Smilowitz2013} (Workforce management in periodic delivery
operations, Smilowitz 2013) address periodic VRP in the context of driver regularities for improving efficiency. compare a two stage approach (routes first driver assignment second) to an integrated approach

\TODO{Papers on periodic maintenance / service technician routing? Papers referenced in \cite{Matl2017}}

\subsubsection*{Orienteering problems}

Orienteering problems explicitly focus on the selection and routing of customers such that a profit measure is maximal.
There is a rich body of work in this line of research.
We limit ourselves to an overview of the most relevant models and publications and refer to the surveys in \cite{Vansteenwegen2011} and \cite{Gunawan2016} for a more extensive overview.

The problem closest related to our application is the multi-period orienteering problem with multiple time windows (MuPOPTW) introduced in \cite{Tricoire2010}.
The authors address a setting where sales representatives schedule visits on a weekly basis subject to daily working time limitations such that the profits assigned to the selected optional customers are maximal. 
In contrast to our application, regularities are not considered in the model.
Instead, regular customers that are frequently served are modeled as mandatory customers.
In each planning period, customers are only served once. 
The authors propose a variable neighborhood search for solving this problem.
%An initial solution is built by sequentially inserting visits into emerging vehicle routes in two stages:
%First, only mandatory visits are inserted this ways. 
%The routes constructed this way are then completed with optional customer visits.
%The VNS uses a cross-exchange neighborhood to improve routes, an optional exchange neighborhood to change the optional customers, and a 3-opt*  for local improvements.
They solve instances with up to 12 mandatory and 140 optional customers modeled after a real-world use case.

A closely related problem in the context of planning tourist trips is addressed in \cite{Kotiloglu2017}.
In this setting, tourist trips over several days are planned based on a set of mandatory visits selected by the tourist and optional visit suggested by a recommender system. 
This recommender system serves as a filter for selecting a subset of options out of the total set of tourist destinations. 
Then, the problem of planning tours over several days based on the mandatory destinations and suggested optional visits such that a profit measure is maximized is modeled as a MuPOPTW.
The problem is solved using an iterated tabu search embedded in a multi-start approach. 

\cite{Qin2015} introduce the multi-period inspector scheduling problem (MPISP).
This problem involves planning trips for inspectors over the course of several days with the objective of maximizing the total workload associated with the selected visits.
Neither mandatory customers or periodic aspects are considered. 
The problem is solved using a tabu search heuristic.

\cite{Stavropoulou2019} introduce the consistent vehicle routing problem with profits (ConVRP).
This problem considers a planning horizon comprising several planning periods.
Customers may require several visits in predefined periods.
Additionally, optional visits can be performed in each period, each one yielding a given profit value.
The objective is to plan tours such that capacity and duration constraints are respected, the customers that require several visits are served by the same vehicle in each period, and the total profit is maximal. 
The problem is solved using an adaptive tabu search procedure.
Unlike our model, this model addresses the aspect of assigning customers to salespersons.
However, while some customers may require several visits, it does not involve the selection of a visit pattern or schedule, instead relying on a predefined visit day assignment.

\subsection*{Summary and comparison}

\TODO{distinguish between daily workload restrictions and daily workload balance in the table!}

\begin{center}
\begin{table}[htbp]
\footnotesize
\begin{tabularx}{\textwidth}{XXXXXX} 
\hline
Reference & Multi-period & Compactness & Daily workload & Profits & Regularities \\
\hline
\cite{Lei2015} & x & x & x (penalized overtime) & - & - \\
\cite{Bender2016} & x & x & - & - & x \\
\cite{Tricoire2010} & x & - & x & x & - \\
\cite{Kotiloglu2017} & x & - & x & x & - \\
\cite{Qin2015} & x & - & x & x & - \\
\cite{Stavropoulou2019} & x & - & x & x & - \\
\hline
This contribution (tactical level) & x & x & x & x & x  \\
This contribution (operational planning) & x & - & x & x & x  \\
\hline
\end{tabularx}
\caption{Model comparison} \label{table:model_comparison}
\end{table}
\end{center}

Problems related to our setting have been proposed in the domains of territory design and vehicle routing.
Generally speaking, territory design addresses the problem on a tactical level.
The objective in this case is to determine balanced groups of customers that minimize a geographical compactness measure.
The strength of these models is the explicit consideration of balance criteria and geographical aspects. 
Vehicle routing instead addresses the operational aspect of planning customer sequences subject to e.g. route duration or working time restrictions, which are difficult to represent accurately in territory design.
However, these problem variants only implicitly favor (day) compactness, as efficient routes often involve visiting compact groups of customers to reduce overall travel time.
%Additionally, the literature has typically focused on either profit maximization in generalizations of the orienteering problem, or the problem of scheduling periodic customer visits. 

Due to the complexity of the different planning problems, all authors propose heuristics for solving problem instances with realistic sizes.
The problem formulations that involve a routing subproblem, i.e. vehicle routing or orienteering problem variants as well as the MTSPDPMPMD, are typically solved using local search heuristics such as VNS, ALNS or tabu search.
For MPSTDP, an exact approach as well as a location allocation heuristic have been proposed.
However, only the latter is able to solve realistic problem instances.

\section*{Modeling the problem}

We first introduce the fundamental models for planning profitable tours with optional client.
Based on these basic formulations, we then discuss different input data modeling variants.

\subsection*{Basic model variants}

We introduce two mixed integer modeling variants for planning profitable tours:
First, we model the problem as a variant of the multi-period service territory design problem (MPSTDP) introduced in \cite{Bender2016}.
We then give the model as a periodic orienteering problem with time windows (POPTW).
Table \ref{table:common_parameters} introduces the problem parameters and sets that used in all modeling variants.

%\comment{unified terminology: in both models, refer to 'clients' instead of 'basic areas' (as in territory design) or 'customers' (in VRP). Use 'profit' instead of 'reward'. But what do we call the center?}

\begin{center}
\begin{table}[htbp]
\begin{tabular}{l l} 
\hline
Sets & \\
\hline
$B$ & clients \\
$B^+ = B \cup \{n\}$  & clients and sales representative location\\
$W$ & weeks in the planning horizon \\ 
$D$ & days in the planning horizon \\
$D_w \subset D$ & days included in week $w$ \\
\hline
Parameters & \\
\hline
$n$ & `depot': starting and ending location of the daily tours \\
$c_{bb'}$ & distance between $b,b' \in B^+$\\
$t_{bb'}$ & driving time between $b,b' \in B^+$\\
$t^{service}_b$ & service time for client $b$\\
$r_b$ & profit associated with each visit at client $b$\\
$m_b$ & number of visits at $b$ per week\\
\hline
\end{tabular}
\caption{Common model sets and parameters} \label{table:common_parameters}
\end{table}
\end{center}

\subsubsection*{Territory design based modeling variant}

\begin{center}
\begin{table}[htbp]
\begin{tabular}{l l} 
\hline
Sets and parameters & \\
\hline
$P_b$ & valid week patterns for client $b \in B$, indexed $p$ \\
$Q_b$ & valid weekday patterns for client $b \in B$, indexed $q$\\
$\mu_d$ & desired workload for day $d \in D$\\
$\mu_w = \sum_{d \in D_w}\mu_d$ & workload for week $w \in W$\\
$\hat{t}_b$ &  driving time estimate for client $b$ \\
$\tau^{day}$ & weekday balance (max deviation)\\
$\tau^{week}$ & week balance (max deviation)\\
$\phi(d) \in W$ & week of day $d$\\
$\omega(d,q)$ & equals 1 if day $d$ is part of weekday pattern $q$\\
$\psi(w,p)$ & equals 1 if week $w$ is part of week pattern $p$\\
$v^{min}$ & minimum number of visits per day\\
$\lambda^{DC}, \lambda^{WC}, \lambda^{prio}, \lambda^{exc}, \lambda^{sav}$ & weights in objective function \\
\hline
Decision variables & \\
\hline
$g_{bp} \in \{0, 1\}$ & equals 1 iff week pattern $p$ selected for client $b$\\
$h_{bqw} \in \{0, 1\}$ & equals 1 iff weekday pattern $q$ selected in week $w$\\
$y_{db} \in \{0, 1\}$ & equals 1 iff $b$ is weekday center on day $d$\\
$\gamma_{wb} \in \{0, 1\}$ & equals 1 iff $b$ is week center in week $w$\\
$\alpha_{bcw} \in \{0, 1\}$ & equals 1 iff $b$ is assigned to week center $c$ in week $w$\\
$\beta_{bcd} \in \{0, 1\}$ & equals 1 iff $b$ is assigned to day center $c$ on day $d$\\
\hline
\end{tabular}
\caption{Additional sets, parameters and decision variables for the territory design approach} \label{table:territory_parameters}
\end{table}
\end{center}

The additional sets and parameters as well as the decision variables are given in Table \ref{table:territory_parameters}.
For all clients $b$, feasible schedules are defined by the set of valid week patterns $P_b$ and the set of weekday patterns $Q_b$.
For each week, $\psi(w,p)$ is 1 if week $w \in W$ is part of pattern $p \in P_b$ and 0 otherwise. Similarly, $\omega(d,q)$ indicates whether day $d \in D$ is included in pattern $q \in Q_d$. 
As the territory design problem does not specify a sequence of customers, we use a sequence-independent travel time estimate $\hat{t}_b$ for clients $b \in B$ that depends on the average driving time to the clients' neighbors.
The daily workload includes these travel time estimates as well as the service times of all clients visited on the respective day.
Workload is limited by and balanced with respect to a desired daily workload $\mu_d$ and a desired weekly workload $\mu_w$. 
Similar to \cite{Bender2016}, we use the following decision variables: 
\begin{align}
&g_{bp} = 1 \text{ if week pattern } p \text{ selected for client } b, \text{0 otherwise} \notag\\
&h_{bqw}= 1 \text{ if weekday pattern } q \text{ selected for client } b \text{ in week } w, \text{0 otherwise} \notag
\end{align}
Day and week cluster centers are indicated by decision variables:
\begin{align}
&\gamma_{wb} = 1 \text{ if client } b \text{ is week center in week } w, \text{0 otherwise} \notag\\
&y_{db} = 1 \text{ if client } b \text{ is weekday center on day } d, \text{0 otherwise} \notag
\end{align}
Clients are assigned to week and weekday centers using the following variables:
\begin{align}
&\alpha_{bcw} = 1 \text{ if client } b \text{ is assigned to week center } c \text{ in week } w, \text{0 otherwise} \notag\\
&\beta_{bcd} = 1 \text{ if client } b \text{ is assigned to weekday center } c \text{ on day } d, \text{0 otherwise} \notag
\end{align}

Using these additional notations, we can formulate the problem as follows:

\begin{equation}
\lambda^{WC} \sum\limits_{b \in B} \sum\limits_{i \in B} \sum\limits_{w \in W} m_b c_{ib} \alpha_{biw} 
+ \lambda^{DC} \sum\limits_{b \in B} \sum\limits_{i \in B} \sum\limits_{d \in D} c_{ib} \beta_{bid}  
- \lambda^{prio} \sum_{b \in B} \sum_{p \in P_b} \sum_{w \in W} m_b \psi(w,p) r_b g_{bp}  
\rightarrow \text{min} \label{territory_model:obj}
\end{equation}
s.t.
\begin{align}
&\sum\limits_{p \in P_b} g_{bp} \leq 1 ~~ b \in B \label{territory_model:wpa} \\
&\sum\limits_{i \in B} \alpha_{biw} = \sum\limits_{p \in P_b} \psi(w,p) g_{bp}  ~~  b \in B, w \in W \label{territory_model:wa} \\
&\alpha_{ibw} \leq \gamma_{wi}  ~~  b,i \in B, w \in W \label{territory_model:only_wc} \\
&\sum\limits_{b \in B} \gamma_{wb} = 1  ~~  w \in W \label{territory_model:wc} \\
&\sum_{d \in D_w}\sum_{b \in B}(t_{nb} + t_{bn})y_{db} + 
\sum_{b \in B} \sum_{p \in P_b} m_b (t^{service}_b + \hat{t}_b) \psi(w,p) g_{bp} 
\geq (1 - \tau^{week})\mu_{w}   ~~  w \in W \label{territory_model:target_weekly_workload_lb}\\
&\sum_{d \in D_w}\sum_{b \in B}(t_{nb} + t_{bn})y_{db} + 
\sum_{b \in B} \sum_{p \in P_b} m_b (t^{service}_b + \hat{t}_b) \psi(w,p) g_{bp}
\leq (1 + \tau^{week})\mu_{w}   ~~  w \in W \label{territory_model:target_weekly_workload_ub} \\
&\sum\limits_{q \in Q_b} h_{bqw} = \sum\limits_{p \in P_b} \psi(w,p) g_{bp}  ~~  b \in B, w \in W \label{territory_model:link_wp_wdp} \\
&\sum\limits_{i \in B} \beta_{bid} = \sum\limits_{q \in Q_b} \omega(d,q) h_{bq\phi(d)}  ~~  b \in B, d \in D \label{territory_model:da} \\
&\beta_{bid} \leq y_{id}  ~~  b,i \in B, d \in D \label{territory_model:only_dc} \\
&\sum\limits_{b \in B} y_{bd} = 1  ~~  d \in D \label{territory_model:dc} \\
&\sum_{b \in B}(t_{nb} + t_{bn})y_{db} + 
\sum_{b \in B} \sum_{q \in Q_b} (t^{service}_b + \hat{t}_b) \omega(d,q) h_{bq\phi(d)}
\geq (1 - \tau^{day})\mu_{d}   ~~  d \in D \label{territory_model:target_daily_workload_lb}\\
&\sum_{b \in B}(t_{nb} + t_{bn})y_{db} + 
\sum_{b \in B} \sum_{q \in Q_b} (t^{service}_b + \hat{t}_b) \omega(d,q) h_{bq\phi(d)}
\leq (1 + \tau^{day})\mu_{d}   ~~  d \in D \label{territory_model:target_daily_workload_ub}\\
&g_{bp} \in \{0,1\}  ~~  b \in B, p \in P_b \label{territory_model:var_wp}\\
&h_{bqw} \in \{0,1\}  ~~  b \in B, q \in Q_b, w \in W \label{territory_model:var_wdp} \\
&\alpha_{biw} \geq 0  ~~  b,i \in B, w \in W \label{territory_model:var_wa} \\
&\beta_{bid} \geq 0  ~~  b,i \in B, d \in D \label{territory_model:var_da} \\
&\gamma_{bw} \in \{0,1\}  ~~  b \in B, w \in W \label{territory_model:var_wc} \\
&y_{bd} \in \{0,1\}  ~~  b \in B, d \in D \label{territory_model:var_dc}
\end{align}

Objective function (\ref{territory_model:obj}) minimizes a weighted objective function that includes the daily and weekly compactness of the planned clusters and the total priority of the included visits.
Constraints (\ref{territory_model:wpa}) ensure that at most one valid week pattern is selected for each client.
Constraints (\ref{territory_model:wa}) ensure that all clients are assigned to exactly one week center in each visit week, i.e. in each week where at least on visit is scheduled for the client. 
Clients that are not included in a plan, i.e. clients for which no week pattern has been selected, are not assigned to any week center.
Constraints (\ref{territory_model:only_wc}) and (\ref{territory_model:wc}) ensure that exactly one week center for each week is chosen chosen among the clients visited in the corresponding week.
Workload balance with respect to a target weekly workload is enforced by Constraints (\ref{territory_model:target_weekly_workload_lb}) and (\ref{territory_model:target_weekly_workload_ub}).

Week and day patterns are linked by Constraints (\ref{territory_model:link_wp_wdp}) for all clients.
If no week pattern is assigned, no day patterns can be selected for the corresponding client.
Similar to Constraints (\ref{territory_model:wpa}) to (\ref{territory_model:target_weekly_workload_ub}), Constraints (\ref{territory_model:da}) to (\ref{territory_model:target_daily_workload_ub}) enforce correct day center assignments and ensure balanced daily workloads.
Variable domains are set in Constraints (\ref{territory_model:var_wp}) to (\ref{territory_model:var_dc}).

\subsubsection*{Orienteering based modeling variant}

\begin{center}
\begin{table}[htbp]
\begin{tabular}{l l} 
\hline
Sets and parameters & \\
\hline
$S_b$ & valid schedules for client $b$\\
$a(d,s)$ & equals 1 iff day $d$ is part of schedule $s \in S$\\
$[\underline{TW}_{bd}, \overline{TW}_{bd}]$ & service time window of client $b \in B$ on day $d$\\
$[\underline{TW}_{nd}, \overline{TW}_{nd}]$ & working time window of depot $n$ on day $d$ \\
$M \gg 0$ & large value \\
\hline
Decision variables & \\
\hline
$x_{bb'd} \in \{0, 1\}$ & equals 1 iff arc $(b,b')$ with $b,b' \in B^+$ traversed on day $d \in D$\\
$z_{bs} \in \{0, 1\}$ & equals 1 iff schedule $s \in S_b$ selected for client $b \in B$\\
$v_{bd} \in \{0, 1\}$ & equals 1 iff client $b \in B$ visited on day $d$\\
$sos_{bd} \in [\underline{TW}_{bd}, \overline{TW}_{bd}]$ & start of service at $b \in B^+$ on day $d$\\
\hline
\end{tabular}
\caption{Additional sets, parameters and decision variables for the orienteering model} \label{table:vrp_parameters}
\end{table}
\end{center}

The additional parameters and decision variables used in the orienteering model are given in Table \ref{table:vrp_parameters}.
In this model, valid combinations of visit days for all clients $b \in B$ are given as a set of schedules $S_b \subset S_{n_b}$ where $S_{n_b}$ indicates the set of all schedules comprising the required number of $n_b$ visits at $b$.
Then, we can define $S_b$ as:
\begin{align*}
S_b = \{s \in S_{n_b}: \exists p \in P_b, q \in Q_b \text{ with } \psi(\phi(d),p) = 1, \omega(d,q) = 1 \forall d \in D \text{ with } a(d,s)= 1\}
\end{align*}
Daily tours are limited by a daily maximum working time window $[\underline{TW}_{nd}, \overline{TW}_{nd}]$. %and client time windows $[\underline{TW}_{bd}, \overline{TW}_{bd}]$.
The formulation of this problem is based on the model for the PVRP by \cite{Christofides}.
For this, we use the following decision variables:
\begin{align*}
&x_{bb'd} = 1 \text{ if arc } (b,b'), b,b' \in B^+ \text { is traversed on day } d, \text{0 otherwise} \notag \\
&z_{bs} = 1 \text{ if schedule } s \in S_b \text{ is selected for client } b, \text{0 otherwise} \notag \\
&v_{bd} = 1 \text{ if client } b \text{ visited on day  }d, , \text{0 otherwise} \notag 
\end{align*}
The problem itself is formulated as follows:
\begin{align}
&\sum_{d \in D}\sum_{b \in B}v_{bd} r_b \rightarrow \max  \label{orienteering_model:obj}
\end{align}
s.t.
\begin{align}
& \sum_{s \in S_b} z_{bs} \leq 1 ~~ b \in B \label{orienteering_model:select_schedule}\\
& v_{bd} = \sum_{s \in S_b}a(d,s) z_{bs} ~~ b \in B
\label{orienteering_model:link_schedule_and_visit}\\ 
& x_{bid} \leq \frac{v_{bd} + v_{id}}{2} ~~ d \in D, b, i \in B, b\neq i \label{orienteering_model:link_visit_and_arc}\\
& \sum_{b \in B^+} x_{bnd} = 1 ~~ d \in D \label{orienteering_model:single_tour_per_day_1}\\
& \sum_{b \in B} x_{nbd} \leq 1 ~~ d \in D \label{orienteering_model:single_tour_per_day_2}\\
& \sum_{i \in B}x_{bid} = \sum_{i \in B} x_{ibd} ~~ d \in D, b \in B^+ \label{orienteering_model:flow_conservation}\\
& \sum_{i\in B^+} x_{ibd} = v_{bd} ~~ b \in B \label{orienteering_model:link_arc_and_visit}\\
& sos_{bd} + t_b^{service} + t_{bi} - sos_{id} \leq M(1 - x_{bid}) ~~ b,i \in B^+, d \in D\label{orienteering_model:start_of_service} \\
& z_{bs} \in \{0, 1\} ~~ b \in B, s \in S_b \label{orienteering_model:var_zbs}\\
& x_{bid} \in \{0, 1\} ~~ b,i \in B^+, d \in D \label{orienteering_model:var_xbid}	
\end{align}

Objective function (\ref{orienteering_model:obj}) the sum of the priorities associated with performed client visits.
Constraints (\ref{orienteering_model:select_schedule}) ensure that at most one valid schedule is selected for all clients. 
The daily boolean indicators $v_{bd}$ for visited clients are set according to these schedules in Constraints (\ref{orienteering_model:link_schedule_and_visit}).
Constraints (\ref{orienteering_model:link_visit_and_arc}) ensure that arcs are only selected between visited clients, while Constraints (\ref{orienteering_model:single_tour_per_day_1}) and (\ref{orienteering_model:single_tour_per_day_2}) limit the solution to at most one tour per day. 
Together with constraints (\ref{orienteering_model:flow_conservation}), these constraints ensure flow conservation.
Constraints (\ref{orienteering_model:link_arc_and_visit}) ensure that all visited clients as indicated by $v_{bd}$ are included in a tour on the corresponding day.
Constraints (\ref{orienteering_model:start_of_service}) set start of service times for visited clients.
This formulation also serves for subtour elimination.
Constraints (\ref{orienteering_model:var_zbs}) to (\ref{orienteering_model:var_xbid}) are domain constraints.

\subsection*{Input data modeling}

Next, we discuss models that implement the different input data variants introduced in Section \ref{somewhere}.

\subsubsection*{Models with mandatory clients}\label{sec:models_obligatory_clients}

In order to distinguish between different client categories, we refer to the set of optional clients as $B^{o}$ and the set of mandatory clients $B^{m}$.
Note that $B = B^{m} \cup B^{o}$.
In this case, only the set of optional clients is associated with profit values.

\paragraph{Territory design}

In the adapted territory design formulation, only the week pattern assignment is changed in order to ensure that mandatory clients are always included in a solution:
\begin{equation}
\lambda^{WC} \sum\limits_{b \in B} \sum\limits_{i \in B} \sum\limits_{w \in W} m_b c_{ib} \alpha_{biw} 
+ \lambda^{DC} \sum\limits_{b \in B} \sum\limits_{i \in B} \sum\limits_{d \in D} c_{ib} \beta_{bid}  
- \lambda^{prio} \sum_{b \in B^{o}} \sum_{p \in P_b} \sum_{w \in W} m_b \psi(w,p) r_b g_{bp}  
\rightarrow \text{min} \label{territory_model:obj_mandatory}
\end{equation}
s.t.
\begin{align}
&\sum_{p \in P_b} g_{bp} = 1 ~~  b \in B^{m} \label{territory_model:relaxed_week_patterns_1}\\ 
&\sum_{p \in P_b} g_{bp} \leq 1 ~~  b \in B^{o} \label{territory_model:relaxed_week_patterns_2}\\
&(\ref{territory_model:wa}) - (\ref{territory_model:var_dc})\notag
\end{align}

The objective function (\ref{territory_model:obj_mandatory}) accounts for the priority of optional visits, as profit values for mandatory visits do not need to be specified.
Constraints (\ref{territory_model:relaxed_week_patterns_1}) and (\ref{territory_model:relaxed_week_patterns_2}) replace Equations (\ref{territory_model:wpa}).
This formulation differentiates between the two sets of clients. 
For those clients that are considered mandatory, exactly one week pattern has to be assigned.
The remaining constraints which enforce workload balance, center selection, and center assignments are unchanged.

\paragraph{Orienteering}

The orienteering model is adjusted in a very similar fashion to the territory design formulation.
Specifically, we ensure that all visits at mandatory clients are included in the solution.
\begin{align}
&\sum_{d \in D}\sum_{b \in B^{o}}v_{bd} r_b \rightarrow \max  \label{orienteering_model:obj_1}
\end{align}
s.t.
\begin{align}
& \sum_{s \in S_b} z_{bs} = 1 ~~ b \in B^m \label{orienteering_model:select_schedule_mandatory}\\
& \sum_{s \in S_b} z_{bs} \leq 1 ~~ b \in B^o \label{orienteering_model:select_schedule_optional}\\
&(\ref{orienteering_model:link_schedule_and_visit}) - (\ref{orienteering_model:var_xbid})\notag
\end{align}

The objective function (\ref{orienteering_model:obj_1} maximizes the sum of priorities associated with optional clients.
Constraints (\ref{orienteering_model:select_schedule_mandatory}) and (\ref{orienteering_model:select_schedule_optional}) replace Constraint (\ref{orienteering_model:select_schedule}), ensuring that for all mandatory clients, exactly one valid visit schedule is selected.

\subsubsection*{ABC modeling variants}\label{sec:models_abc}

We separate the client set $B$ into hierarchically ranked client groups $B^{A}, B^{B}, B^{C}, ...$, with group A comprising the most highly valued clients.

Implementing an 'ABC' client classification using a hierarchical objective function with sufficiently high profit values for highly prioritized client groups does not require model modifications.
For example, we can ensure that 
\begin{equation}
r_b > \sum_{i \in B^{B}} r_i, b \in B^{A},  \notag
\end{equation}
and so on.

The strictly hierarchical model maximizes the sum of priorities of a given client group X subject to the restriction that all clients that are ranked higher are included in the plan.

In other words, if clients are separated into $n$ groups, we sequentially solve $n$ models based on the variants introduced in Section \ref{sec:models_obligatory_clients}.
For the first model, we set $B^{o} = B^{A}$ and $B^{m} = \emptyset$. 
Assuming all clients of set A can be included, we proceed to solve the model with $B^{o} = B^{B}, B^{m} = B^{A}$ and continue with $B^{o} = B^{C}, B^{m} = B^{A} \cup B^{B}$ etc. until the model becomes infeasible, i.e. until there is no feasible solution that includes all visits in $B^{m}$.
